# Supplementary material for: DeepReDuce: ReLU Reduction for Fast Private Inference
Source: arXiv:2103.01396 source file (2021-06-22)
Supplement: Supplementary file 1 [file 50AppendixTable_StagesInCNNs.tex]

\begin{table} [htbp] \centering
\caption{Stage-wise block structure (repetitions) of ResNet \cite{he2016deep}, ResNeXt \cite{xie2017aggregated}, SENet \cite{hu2018squeeze}, NFNet \cite{brock2021characterizing,brock2021high}, Bottleneck Transformers for Visual Recognition (BoTNet) \cite{srinivas2021bottleneck}, BagNet \cite{brendel2018approximating}, Dual Path Networks (DPN) \cite{chen2017dual}, DenseNet \cite{huang2017densely}, CondenseNet \cite{huang2018condensenet}, MobileNetV2 \cite{sandler2018mobilenetv2}, ShuffleNet \cite{zhang2018shufflenet,ma2018shufflenet}, GoogLeNet \cite{szegedy2015going}, InceptionNet \cite{szegedy2016rethinking,szegedy2017inception}, PolyNet \cite{zhang2017polynet}, Wide Residual Network (WRN) \cite{zagoruyko2016wide}, SqueezeNext (SqNxt) \cite{gholami2018squeezenext}, and RegNet (GF implies GFlops) \cite{radosavovic2020designing}. The numbers in brackets are the number of repetitions of similar blocks withing the stages (i.e. [$S_1$, $S_2$, ..., $S_D$] respectively). For simplicity, we ignore the first conv (stem) layer present just after the inputs. (Bold number represents highest number of repetitions. $^\dag$ represents the models designed for CIFAR-10/100, and In-ResNet is Inception ResNet)}
\label{tab:StagesInDNNs}
\resizebox{.5\textwidth}{!}{
\begin{tabular}{c|c||c|c} \toprule
Networks & \# Repetitions   & Networks & \# Repetitions \\ \toprule
ResNet18  & [2, 2, 2, 2]  & ResNet20$^\dag$   &  [3, 3, 3]  \\
ResNet34 & [3, 4, {\bf 6}, 3]  & ResNet32$^\dag$  &  [5, 5, 5]  \\
ResNet50  & [3, 4, {\bf 6}, 3]  &  ResNet44$^\dag$   &  [7, 7, 7]  \\
ResNet101  & [3, 4, {\bf 23}, 3]  &  ResNet56$^\dag$   &  [9, 9, 9]  \\ 
ResNet152  & [3, 8, {\bf 36}, 3]  &  ResNeXt29$^\dag$  &  [3, 3, 3]  \\
ResNeXt50   &  [3, 4, {\bf 6}, 3] & CondenseNet$^\dag$  & [14, 14, 14]   \\
ResNeXt101  &  [3, 4, {\bf 23}, 3] & ShuffleNetV1 & [4, {\bf 8}, 4] \\
ResNeXt152    &  [3, 8, {\bf 36}, 3] & ShuffleNetV2    & [4, {\bf 8}, 4]   \\
SENet50    &  [3, 4, {\bf 6}, 3] &  GoogLeNet & [2, {\bf 5}, 2]     \\
SENet101    &  [3, 4, {\bf 23}, 3] & InceptionV3 & [3, {\bf 5}, 2] \\
SENet152   &  [3, 8, {\bf 36}, 3] & InceptionV4 & [4, {\bf 7}, 3]  \\
SENet350   &  [4, 40, {\bf 60}, 12] & In-ResNetV1 & [5, {\bf 10}, 5]  \\
NFNet-F0 &  [1, 2, {\bf 6}, 3] &  In-ResNetV2 & [10, {\bf 20}, 10]  \\
NFNet-F1 &  [2, 4, {\bf 12}, 6] & PolyNet & [3, {\bf 6}, 3]   \\
NFNet-F2 &  [3, 6, {\bf 18}, 9] &  WRN-16x2 & [2, 2, 2] \\
NFNet-F3 &  [4, 8, {\bf 24}, 12] & WRN-22x2 & [3, 3, 3] \\
NFNet-F4 &  [5, 10, {\bf 30}, 15] & WRN-28x2 & [4, 4, 4] \\
NFNet-F5 &  [6, 12, {\bf 36}, 18] & WRN-40x2 & [6, 6, 6] \\
NFNet-F6 &  [7, 14, {\bf 42}, 21] & SqNxt-23v2 & [6, 6, {\bf 8}, 1]   \\ 
BoTNet-S1-59  &  [3, 4, {\bf 6}, {\bf 6}] & SqNxt-23v3 & [4, {\bf 8}, {\bf 8}, 1]\\
BoTNet-S1-77  &  [3, 4, 6, {\bf 12}] & SqNxt-23v4 & [2, {\bf 10}, 8, 1] \\
BoTNet-S1-110  &  [3, 4, {\bf 23}, 6] & SqNxt-23v5 & [2, 4, {\bf 14}, 1] \\
BoTNet-S1-128  &  [3, 4, {\bf 23}, 12] & RegNetX-0.2GF & [1, 1, 4, {\bf 7}] \\
BagNet & [3, 4, {\bf 6}, 3]   & RegNetX-0.4GF    &  [1, 2, 7, {\bf 12}] \\
DPN92 & [3, 4, {\bf 20}, 3]  & RegNetX-0.6GF  & [1, 3, 5, {\bf 7}]   \\
DPN98 & [3, 6, {\bf 20}, 3] & RegNetX-0.8GF    & [1, 3, {\bf 7}, 5]   \\
DPN101 & [4, 8, {\bf 20}, 3] & RegNetX-1.6GF  &  [2, 4, {\bf 10}, 2]  \\
DPN137 & [4, 8, {\bf 28}, 3] &   RegNetX-3.2GF    &  [2, 6, {\bf 15}, 2]  \\
DenseNet121  & [6, 12, {\bf 24}, 16]  & RegNetX-4.0GF & [2, 5, {\bf 14}, 2] \\ 
DenseNet169  &  [6, 12, {\bf 32}, {\bf 32}]  & RegNetX-6.4GF & [2, 4, {\bf 10}, 1]\\ 
DenseNet201  &  [6, 12, {\bf 48}, 32]  & RegNetX-8.0GF  & [2, 5, {\bf 15}, 1]   \\
DenseNet264  &  [6, 12, {\bf 64}, 48] &  RegNetX-12GF  & [2, 5, {\bf 11}, 1]   \\
CondenseNet  & [4, 6, 8, {\bf 10}, 8] & RegNetX-16GF  & [2, 6, {\bf 13}, 1]    \\
MobileNetV2  & [1, 2, 3, {\bf 7}, 3]  &  RegNetX-32GF  &  [2, 7, {\bf 13}, 1]   \\ 
\bottomrule
\end{tabular} }
\end{table}
